# Supplementary material for: Textless Direct Speech-to-Speech Translation with Discrete Speech Representation
Source: arXiv:2211.00115 source file (2022-10-31)
Supplement: Supplementary file 1 [file 9-appendix.tex]

\appendix
\onecolumn

\begin{landscape}

\section{Detailed evaluation results of the S2ST models}
\label{a:eval-details}

\begin{table*}[h]
\centering
\begin{small}
\footnotesize
\caption{Performance of the multilingual X$\to$En S2ST models on CVSS-C test sets. Evaluated by BLEU on ASR transcription.}
\setlength{\tabcolsep}{0.45em}
\begin{tabular}{lrrrrrrrrrrrrrrrrrrrrrrrr}
    \toprule
     & \multicolumn{2}{c}{\#Params} & & \multicolumn{4}{c}{High-resource} & \multicolumn{5}{c}{Mid-resource} & \multicolumn{12}{c}{Low-resource} \\
     \cmidrule{2-3}\cmidrule(r){5-8}\cmidrule(lr){9-13}\cmidrule(l){14-25}
    X$\to$En & Encoder & Decoder & Avg & fr & de & ca & es & fa & it & ru & zh & pt & nl & tr & et & mn & ar & lv & sl & sv & cy & ta & ja & id \\
    Hours (source) & & & & 264 & 184 & 136 & 113 & 49 & 44 & 18 & 10 & 10 & 7.3 & 4.1 & 3.4 &  3.0 &  2.1 &  2.1 &  2.0 &  1.7 &  1.7 &  1.6 & 1.3 & 1.2  \\
    
    \midrule
    \multicolumn{4}{l}{\kern-0.5em\emph{From scratch}} \\
    Baselines \citep{jia2022cvss} & 26M & 10M & 8.7 & 28.3 & 19.7 & 23.5 & 30.1 & 2.4 & 24.1 & 19.6 & 4.5 & 12.5 & 6.5 & 3.8 & 0.6 & 0.2 & 1.7 & 1.5 & 0.4 & 1.3 & 0.9 & 0.1 & 0.5 & 0.4 \\
    This work & 26M & 25M & 10.1 & 29.5 & 22.3 & 25.0 & 30.8 &  3.4 & 26.0 & 21.7 &  5.5 & 14.3 & 10.5 &  6.6 &  1.1 &  0.2 &  3.8 &  3.0 &  2.3 &  2.8 &  1.6 &  0.1 &  0.5 &  0.8 \\
    \midrule
    \multicolumn{4}{l}{\kern-0.5em\emph{Encoder pre-training}} \\
    Speech & 0.6B & 25M & 17.9 & 33.6 & 30.6 & 30.1 & 35.9 &  6.0 & 32.5 & 38.9 &  5.2 & 31.9 & 29.3 &  9.2 & 16.0 &  0.2 & 10.4 & 15.6 & 17.8 & 25.9 &  4.2 &  0.3 &  0.9 &  1.5 \\
    Speech + Text & 0.6B & 25M & 17.8 & 34.5 & 30.7 & 31.1 & 36.9 &  5.9 & 33.8 & 38.1 &  4.0 & 31.1 & 28.6 &  8.1 & 15.0 &  0.2 &  7.0 & 16.0 & 18.6 & 28.1 &  3.5 &  0.2 &  0.9 &  1.3 \\
    Speech + Text & 0.6B & 113M & 18.1 & 34.9 & 31.1 & 31.7 & 37.0 &  4.6 & 34.0 & 38.3 &  3.8 & 33.3 & 30.6 &  7.1 & 15.0 &  0.2 &  5.8 & 17.4 & 20.8 & 29.0 &  2.7 &  0.3 &  0.8 &  1.1 \\
    % EPT (S-T, 1.8B) & 19.2 & 32.6 & 30.0 & 29.4 & 34.6 &  8.9 & 31.9 & 40.2 &  5.0 & 35.6 & 29.3 & 19.9 & 17.8 &  0.2 & 14.5 & 16.5 & 21.5 & 29.4 &  3.2 &  0.3 &  1.1 &  2.0 \\
    Speech + Text & 1.8B & 25M & 20.2 & 35.4 & 31.6 & 31.6 & 36.9 & 10.4 & 34.8 & 40.1 &  3.3 & 40.1 & 32.2 & 17.3 & 16.9 &  0.1 &  9.9 & 21.6 & 24.7 & 33.4 &  1.6 &  0.1 &  0.5 &  1.0 \\
    \midrule
    \multicolumn{4}{l}{\kern-0.5em\emph{Decoder pre-training}} \\
    Text-to-text & 26M & 25M & 9.6 & 28.9 & 21.6 & 24.5 & 30.7 &  2.8 & 25.0 & 21.4 &  5.6 & 13.1 &  8.6 &  6.2 &  1.0 &  0.2 &  2.8 &  1.9 &  1.7 &  1.5 &  1.6 &  0.2 &  0.6 &  0.8 \\
    Text-to-phoneme & 26M & 25M & 10.1 & 29.5 & 22.0 & 25.3 & 30.5 &  3.8 & 25.3 & 22.4 &  4.9 & 15.6 & 10.5 &  7.3 &  0.8 &  0.2 &  4.1 &  2.6 &  3.2 &  2.2 &  1.0 &  0.1 &  0.8 &  1.0 \\
    Phoneme-to-phoneme & 26M & 25M & 9.9 & 29.2 & 22.0 & 24.5 & 30.4 &  3.7 & 25.1 & 22.4 &  5.6 & 11.7 &  9.8 &  7.3 &  1.0 &  0.2 &  4.0 &  2.1 &  2.3 &  3.0 &  1.3 &  0.2 &  0.7 &  1.4 \\
    \midrule
    \multicolumn{4}{l}{\kern-0.5em\emph{Multi-task fine-tuning}} \\
    $\tau_\textrm{MT}=1.0$ & 0.6B & 25M & 19.1 & 35.3 & 32.0 & 31.7 & 37.7 &  6.9 & 34.5 & 41.5 &  5.1 & 33.1 & 31.0 & 10.9 & 16.6 &  0.2 &  7.9 & 17.3 & 23.7 & 31.9 &  2.7 &  0.1 &  0.7 &  1.2 \\
    $\tau_\textrm{MT}=5.0$ & 0.6B & 25M & 19.3 & 33.9 & 31.5 & 30.6 & 36.8 &  7.2 & 33.7 & 41.6 &  6.4 & 34.1 & 31.1 & 16.1 & 17.1 &  0.3 & 10.0 & 14.4 & 22.9 & 28.4 &  5.4 &  0.2 &  1.3 &  2.5 \\
    $\tau_\textrm{MT}=5.0$ & 1.8B & 113M & 22.8 & 34.8 & 32.7 & 31.5 & 36.8 &  9.6 & 34.4 & 44.9 &  7.2 & 40.8 & 34.1 & 24.9 & 21.5 &  0.5 & 20.1 & 21.3 & 26.3 & 34.1 &  4.6 &  0.4 &  1.5 & 16.0 \\
    \midrule
    \multicolumn{4}{l}{\kern-0.5em\emph{TTS-based data aug.}} \\
    $\tau_\textrm{aug}=1.0$ & 0.6B & 25M & 19.7 & 35.0 & 32.2 & 31.1 & 37.2 &  5.9 & 33.8 & 43.2 & 11.4 & 33.0 & 29.8 & 11.7 & 16.6 &  0.4 & 11.2 & 15.5 & 22.7 & 30.1 &  4.0 &  0.1 &  5.7 &  2.9 \\
    $\tau_\textrm{aug}=1.0$ & 1.8B & 113M & 23.5 & 36.0 & 33.7 & 31.8 & 38.2 &  8.2 & 35.3 & 46.1 & 15.0 & 39.4 & 33.5 & 23.4 & 20.8 &  0.2 & 19.2 & 21.9 & 26.3 & 33.5 &  3.4 &  0.3 &  9.5 & 18.2 \\
    $\tau_\textrm{aug}=5.0$ & 0.6B & 25M & 22.0 & 34.5 & 32.0 & 30.7 & 37.1 &  8.2 & 33.8 & 42.6 & 10.6 & 34.0 & 31.8 & 23.9 & 17.2 &  1.1 & 22.4 & 15.6 & 23.3 & 31.1 &  7.6 &  0.6 &  5.5 & 18.5 \\
    $\tau_\textrm{aug}=5.0$ & 0.6B & 113M & 22.1 & 35.7 & 32.0 & 31.6 & 37.8 &  5.9 & 35.0 & 42.4 &  9.0 & 36.9 & 32.0 & 21.0 & 16.9 &  0.6 & 19.5 & 18.5 & 25.4 & 32.7 &  4.3 &  0.4 &  4.0 & 22.0 \\
    $\tau_\textrm{aug}=5.0$ & 1.8B & 113M & 25.6 & 36.5 & 33.6 & 31.9 & 38.5 & 11.6 & 35.7 & 45.6 & 13.1 & 41.1 & 34.1 & 28.7 & 21.0 &  2.5 & 30.2 & 22.7 & 25.8 & 36.6 &  5.4 &  2.2 &  8.5 & 32.8 \\

    % DPT (P-P) \\
    % EPT (S, 0.6B) + DPT (P-P) \\
    % EPT (S-T, 0.6B) + DPT (P-P) + MFT \\
    % EPT (S-T, 2B) + DPT (P-P) + MFT \\
    
    \iffalse
    \midrule
    \multicolumn{4}{l}{\kern-0.5em\emph{Cascade (ST $\to$ TTS)}} \\
    Baseline \citep{jia2022cvss} & 10.6 & 31.2 & 23.9 & 26.8 & 33.3 & 3.4 & 28.1 & 24.4 & 6.8 & 14.8 & 9.8 & 5.1 & 1.7 & 0.3 & 4.1 & 2.3 & 0.6 & 1.4 & 2.1 & 0.2 & 0.7 & 0.9 \\
    EPT (S, 0.6B) & 19.7 & 36.1 & 33.1 & 32.7 & 38.3 & 5.4 & 35.4 & 41.0 & 5.2 & 37.6 & 32.9 & 8.0 & 17.0 & 0.3 & 11.0 & 16.4 & 25.2 & 30.9 & 4.3 & 0.3 & 0.7 & 2.4 \\
    EPT (S-T, 0.6B) + MFT & 21.6 & 37.1 &  35.6 &  33.8 &  39.7 &   7.4 &  36.8 &  46.3 &   8.1 &  36.3 &  34.7 &  15.8 &  19.5 &   0.8 &  13.2 &  18.4 &  23.7 &  30.8 &   7.2 &   0.6 &   2.4 &   5.0 \\
    EPT (S-T, 2B) + MFT & 23.3 & 37.6 & 35.7 & 33.7 & 39.9 & 10.9 & 37.0 & 47.5 &  6.6 & 42.5 & 35.6 & 23.4 & 21.7 &  0.7 & 18.2 & 22.6 & 28.3 & 35.8 &  4.5 &  0.4 &  1.5 &  5.4 \\
    \fi
    
    \midrule
    \emph{Prior state-of-the-art \citep{jia2022cvss}} & 26M & 10M & 12.0 & 32.4 & 24.8 & 28.2 & 33.4 & 6.3 & 28.6 & 23.2 & 6.3 & 18.3 & 15.8 & 10.6 & 2.5 & 0.4 & 5.4 & 2.3 & 3.1 & 3.2 & 4.5 & 0.1 & 1.0 & 1.0 \\
    
    \midrule
    \emph{Reference} & & & 91.1 & 84.6 & 88.4 & 92.0 & 88.6 & 91.7 & 89.5 & 94.0 & 77.8 & 93.1 & 90.6 & 92.7 & 89.3 & 92.4 & 94.2 & 94.8 & 94.9 & 94.1 & 92.0 & 90.6 & 95.3 & 92.6 \\
    \bottomrule
\end{tabular}
\label{tbl:eval-details}
\end{small}
\end{table*}

\newpage

\section{Amount of the MT dataset and the TTS-augmented S2ST dataset}
\label{a:data-details}

\begin{table*}[h]
\centering
\begin{small}
\footnotesize
\caption{Amount of source data in the MT dataset and the TTS-augmented S2ST dataset.}
\setlength{\tabcolsep}{0.45em}
\begin{tabular}{lrrrrrrrrrrrrrrrrrrrrrc}
    \toprule
     & \multicolumn{4}{c}{High-resource} & \multicolumn{5}{c}{Mid-resource} & \multicolumn{12}{c}{Low-resource} & \multirow{2.5}{*}{Total} \\
     \cmidrule(r){2-5}\cmidrule(lr){6-10}\cmidrule(l){11-22}
     & fr & de & ca & es & fa & it & ru & zh & pt & nl & tr & et & mn & ar & lv & sl & sv & cy & ta & ja & id \\
    \midrule
    MT ($\times 10^3$ sentences) & 38,288 & 38,363 & 96 & 13,134 & 205 & 236 & 33,512 & 22,200 & 61 & 191 & 210 & 2,152 & 10 & 216 & 623 & 22 & 59 & 1 & 738 & 17,879 & 89 & 168,285 \\
    S2ST (hours) & 103,157 & 82,037 & 97 & 37,240 & 397 & 397 & 81,637 & 46,511 & 92 & 286 & 539 & 3,796 & 13 & 443 & 1,553 & 34 & 80 & 1 & 1,413 & 39,102 & 156 & 398,983 \\
    \bottomrule
\end{tabular}
\label{tbl:data-details}
\end{small}
\end{table*}

\end{landscape}

\iffalse

\begin{table}[t]
  \small
  % \footnotesize
  \caption{Comparison between direct and cascade S2ST. (EPT/DPT: encoder/decoder pre-training; MFT: multitask fine-tuning; S: speech; S-T: speech and text.) TODO: put direct and cascade on the same rows.}
%   \caption{S2ST BLEU on CVSS-C when part of the model is pre-trained in ASR/ST tasks on CoVoST~2. Row 4/5 means initializing the encoder and decoder of Translatotron 2 from the ST models used in row 1/2.}
  \label{tbl:pretraining}
  \centering
\begin{tabular}{lrrrr}
    \toprule
    & All & High & Mid& Low \\
    \midrule
    \multicolumn{4}{l}{\kern-0.5em\emph{Direct (Translatotron 2)}} \\
    From scratch                & 10.0 & 27.4 & 14.3 & 2.4 \\
    EPT (S, 0.6B)               & 18.8 & 34.9 & 24.0 & 11.3 \\
   % EPT (S, 0.6B) + DPT         &   &\\
    EPT (S-T, 0.6B) + DPT + MFT & \\
    EPT (S-T, 2B) + DPT + MFT   & \\
    % \midrule
    % Cascade (ST + TTS) & 9.9 & 27.5 & 5.8 \\
    % \quad$+$ ASR pre-training & 12.2 & 30.3 & \\
    % \midrule
    % Translatotron 2 & 8.5 & 25.3 & 4.5 \\
    % \quad$+$ ST pre-training & 10.0 & 27.4 \\
    % \quad\quad$+$ ASR pre-training & 11.6 & 29.7\\
    \midrule
    \multicolumn{4}{l}{\kern-0.5em\emph{Cascade (ST $\to$ TTS)}} \\
    From scratch \citep{jia2022cvss} & 10.6 & 28.8 & 15.5 & 2.4  \\
    EPT (S, 0.6B) & 19.7 & 35.1 & 24.9 & 12.5 \\
    EPT (S-T, 0.6B) + MFT & 21.6 & 36.6 & 27.0 & 14.3 \\
    EPT (S-T, 2B) + MFT & 23.3 & 36.7 & 28.9 & 16.5 \\
    % w2v-bert-51 (0.6B) \citep{bapna2022mslam} & \\
    % sSLAM-CTC (0.6B)  \citep{bapna2022mslam} & \\
    % mSLAM-CTC (2B) \citep{bapna2022mslam} \\
    \midrule
    Reference & 91.1 & 88.4 & 89.2 & 92.8 \\
    \bottomrule
\end{tabular}
\end{table}

\fi
